# Supplementary material for: Receding Hamiltonian-Informed Optimal Neural Control and State Estimation for Closed-Loop Dynamical Systems
Source: arXiv:2411.01297 source file (2025-07-29)
Supplement: Supplementary file 1 [file ap-appendix.tex]

\section{Additional Results}

In addition to the ones presented in Section \ref{sect:hion-results}, we have included some additional simulations conducted with our proposed T-mano controller for distinct scenarios.

\subsection{Stabilization of Second-Order Linear System}
Figure \ref{gr:hion-linear-stable} shows the system dynamics when controlled by the T-mano model to stabilize a second-order linear system that has an initial speed.

\begin{figure}[!hbt]
  \centering
  \includegraphics[width=\textwidth]{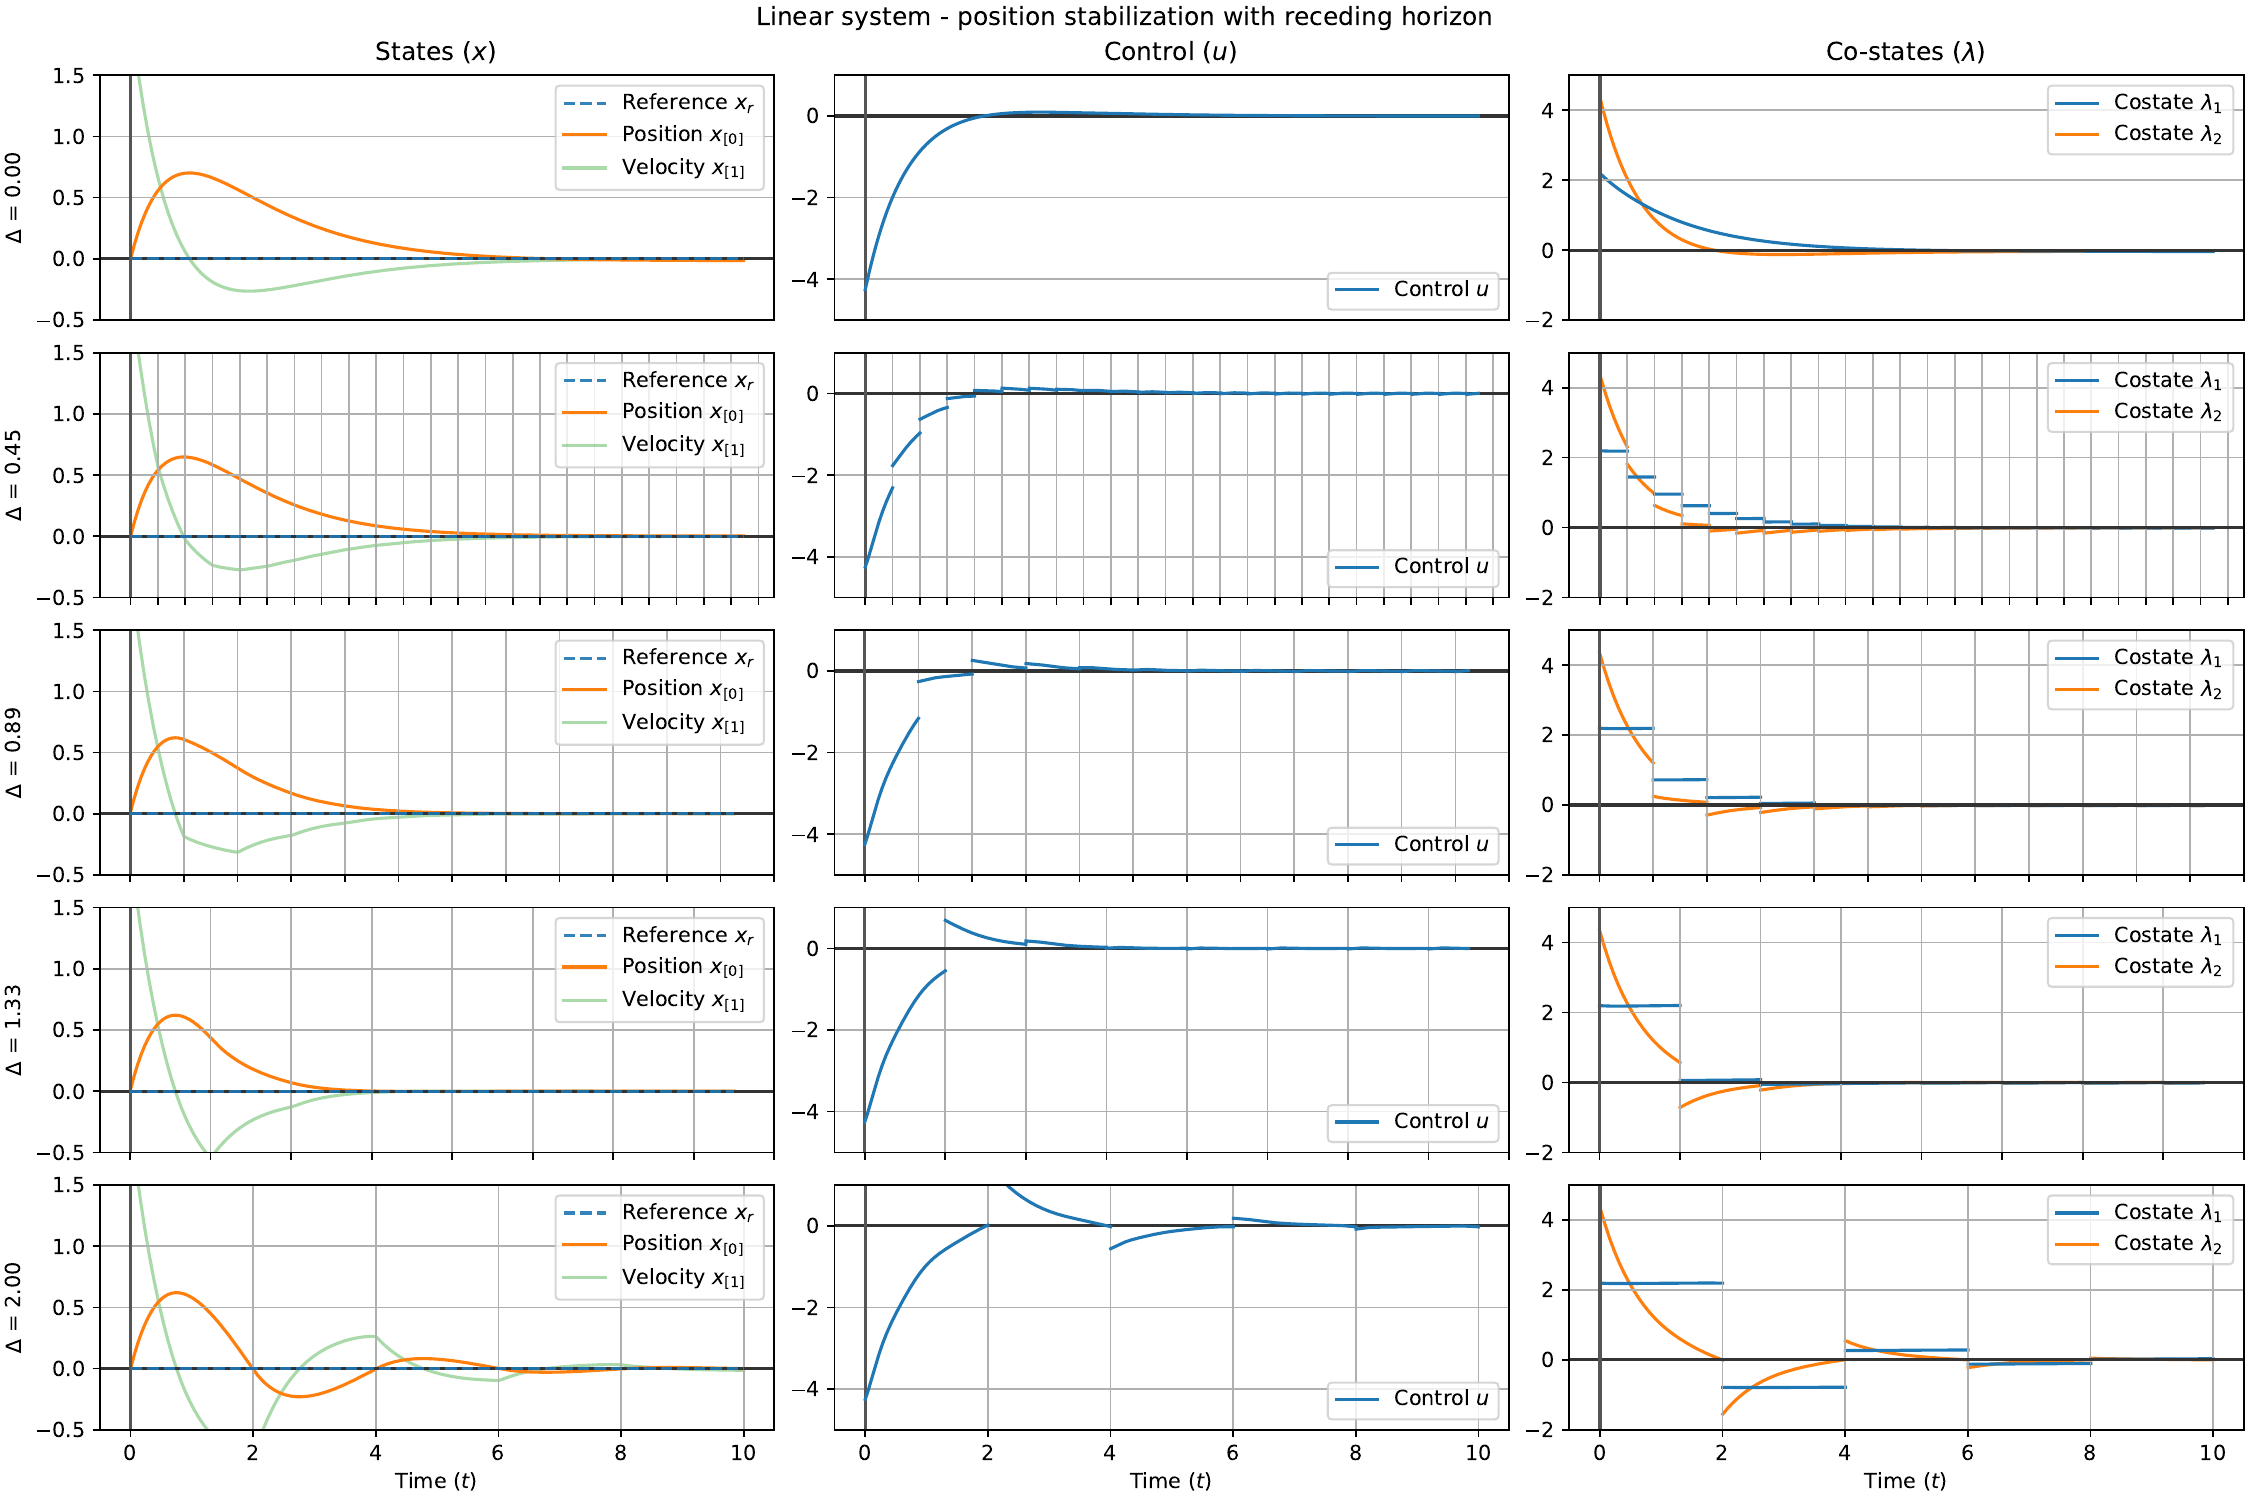}
  \caption{Same linear system controller stabilizing system at different sampling rates.}
  \label{gr:hion-linear-stable}
\end{figure}

\subsection{Model-Predictive Control for Minimal Speed of Van der Pol oscillator}

Figure \ref{gr:hion-van-speed} showcases the various dynamics for a Van der Pol oscillator when the environment states are observed at different sampling rates.

\begin{figure}[!hbt]
  \centering
  \includegraphics[width=\textwidth]{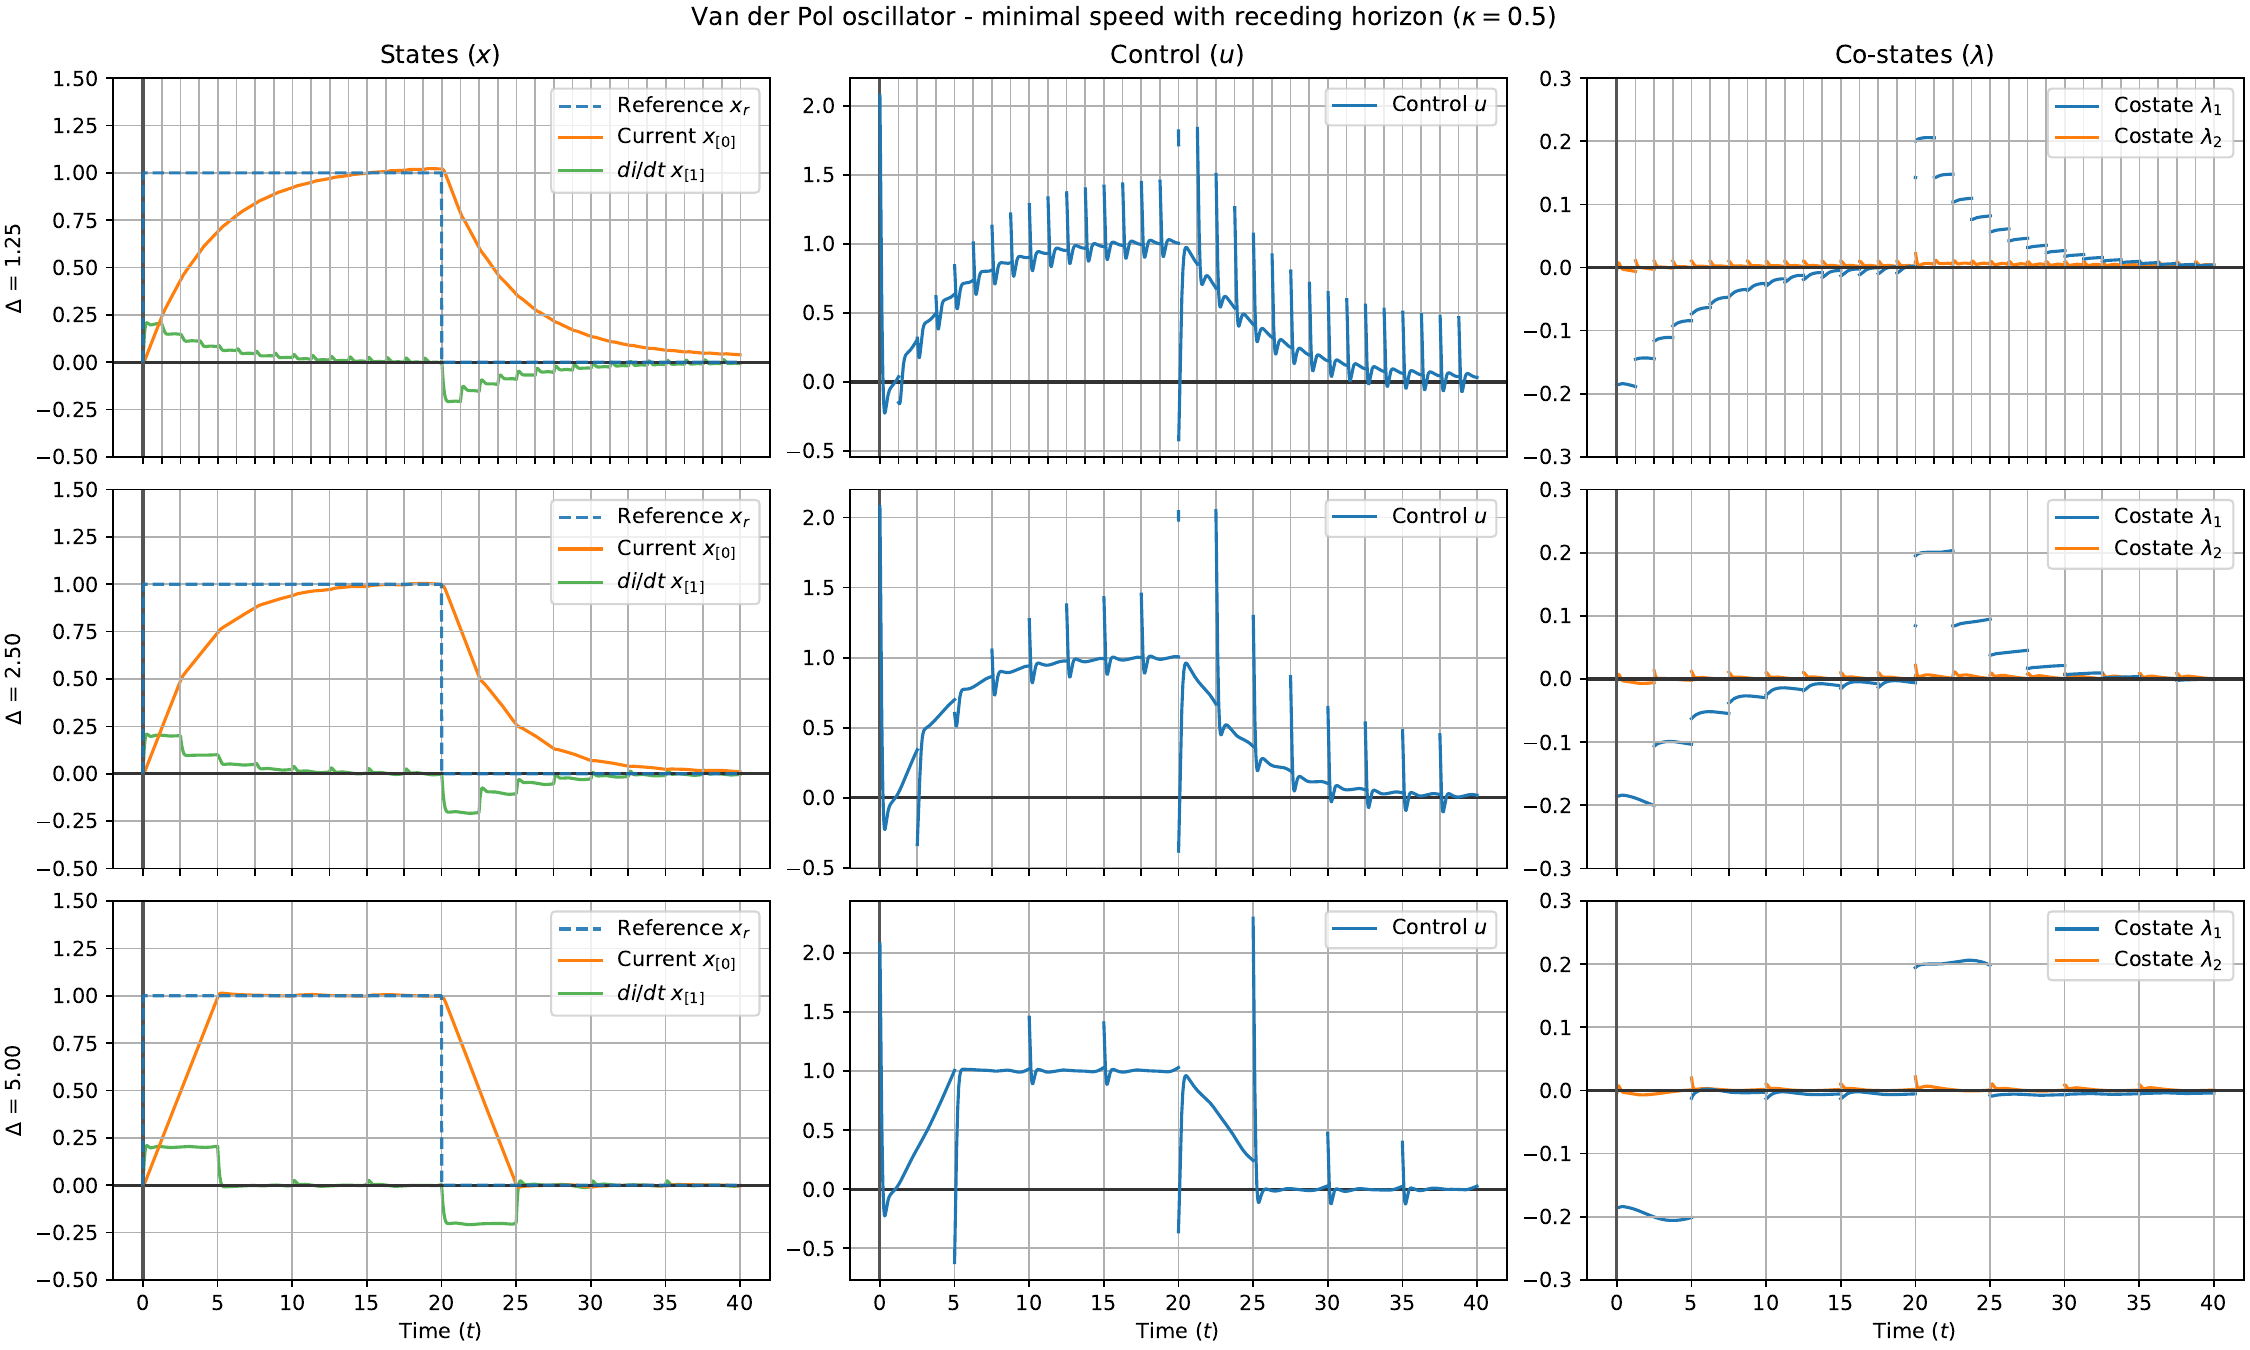}
  \caption{Same Van der Pol system controller for reduced speed at different sampling rates.}
  \label{gr:hion-van-speed}
\end{figure}
